# Supplementary material for: Classification-Regression for Chart Comprehension
Source: arXiv:2111.14792 source file (2022-07-11)

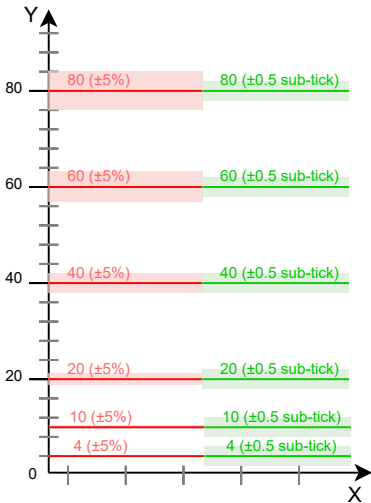

Supplement: Supplementary file 1 [file tick_vs_ratio_metric.pdf]
